# Supplementary material for: Competitive DER Aggregation for Participation in Wholesale Markets
Source: arXiv:2207.00290 source file (2022-07-01)
Supplement: Supplementary file 1 [file appendixProofTHM2_v8.tex]

% (\ref{eq:ProfitMaxDirect}) is the profit maximization of the individual prosumer when it directly participate in the wholesale market.

Solving (\ref{eq:wholesaleDiret}) we have $\dbf^{\mbox{\tiny Direct}}_n, p^{\mbox{\tiny Direct}}_r$ and we know that $\pi_{\mbox{\tiny LMP}}=\lambda^*$. By KKT conditions of  (\ref{eq:wholesaleDiret}), we know 
$$d^{\mbox{\tiny Direct}}_{kn}=\max \{\underline{d}_k,\min \{V_{kn}^{-1}(\pi_{\mbox{\tiny LMP}} ),\bar{d}_k\}\}=d^*_{kn}, \forall k, n,$$
where in $d^*_{kn}$ is computed with (\ref{eq:DERAFixRateGP}). So $\dbf^{*}_n$ is the same as the optimal consumption of the prosumer $n$ when it directly participates in the wholesale market with individual profit maximization (\ref{eq:ProfitMaxDirect}) and market clearing problem  (\ref{eq:wholesaleDiret}).

To satisfy the power balance constraints with social welfare maximization, we have  $p^{\mbox{\tiny Direct}}_l=p^*_l, \forall l$. So 
\beq
\begin{array}{lcl}
S_{{\cal W}}&:=&\sum_nU_n(\dbf^{\mbox{\tiny Direct}}_n)-\sum_lC_l(p^{\mbox{\tiny Direct}}_l)\\
&=&\sum_nU_n(\dbf^*_n)-\sum_lC_l(p^*_l)\\
&=& S_{\tiny {\cal W}\mbox{-DERA}}.
\end{array}
\eeq

To show$$\mbox{\sf SW}_{\mbox{ \tiny Direct}}=\mbox{\sf SW}_{\mbox{ \tiny DERA}}=\mbox{\sf SW}^*.$$

follows directly the KKT conditions of (\ref{eq:wholesaleDiret}) and (\ref{eq:ProfitMaxDirect}), from which we have, $\hat{\dbf}_n$, the optimal consumption of the prosumer $n$ the same as $\dbf^{*}_n$  in (\ref{eq:DERAFixRateGP}). Therefore, when prosumers directly participate in the wholesale market, both the optimal wholesale market dispatch and the optimal social welfare are the same as those when prosumers indirectly participate in the wholesale electricity market through a DERA. 

Furthermore, 
Social welfare is the sum of surpluses for all market participants, including prosumers, traditional elastic load demands, and traditional generators \footnote{The current formulation of the wholesale market in (\ref{eq:wholesaleDiret}) can be extended to include transmission constraints and inelastic demands.}. Denote
\beq
\mbox{\sf SW}(\Dbf, \ebf, \pbf):=\sum_nU_n(\dbf_n)+\sum_sU_s(e_s)-\sum_mC_m(p_m),
\eeq
where $C_m(p_m)$ is the generation cost for traditional generators with index $m$ when the output is $p_m$, and $U_s(e_s)$ is the consumption utility for traditional consumers with index $s$  when the consumption is $e_s$.

The wholesale market clearing problem when all prosumers directly participate in the wholesale market is given by 
\bea\label{eq:wholesaleDiret}
\begin{array}{lrl}
&\underset{\Dbf, \ebf, \pbf, \zbf}{\rm max}&~~ \mbox{\sf SW}(\Dbf, \ebf, \pbf)\\
&  \mbox{subject to} & \mbox{for all $ n , s, m$} \\
&\pi_{\mbox{\tiny LMP}}:&\sum_m p_m-\sum_s e_s-\sum_nz_n=0, \\
&&z_n = \mathbf{1}^\intercal \dbf_n-g_n,\\
% & \eta_i: & \omega^0_i \le P^{NEM}_i,\\
&  &\underline{\dbf}_n \preceq  \dbf_n \preceq  \bar{\dbf}_n,\\
&  &\underline{p}_m\le  p_m\le  \bar{p}_m,\\
&  &\underline{e}_s\le  e_s\le  \bar{e}_s.
\end{array}
\eea
 Let $\hat{\dbf}_n, \hat{p}_m, \hat{e}_s$ be the optimal solution to (\ref{eq:wholesaleDiret}). The optimal social welfare when all prosumers directly participate in the wholesale market is given by
\beq
\mbox{\sf SW}_{\mbox{ \tiny Direct}}:=\sum_nU_n(\hat{\dbf}_n)+\sum_sU_s(\hat{e}_s)-\sum_mC_m(\hat{p}_m).
\eeq
Let $\dbf^*_n, p^*_m, e^*_s$ be the output of traditional resources in the wholesale market when the DERA participates with (\ref{eq:DERAFixRateGP}). Then, the optimal social welfare with DERA's participation on behalf of its customers is given by
\beq
\mbox{\sf SW}_{\mbox{ \tiny DERA}}:=\sum_nU_n(\dbf^*_n)+\sum_sU_s(e^*_s)-\sum_mC_m(p^*_m),
\eeq
which is the same for any $\zeta\geq 0$ in (\ref{eq:DERAsurplus_LnGP}). Note that, different $\zeta$ will influence the social welfare distribution among DERA and prosumers, but not the total amount of social welfare.
