# Supplementary material for: Competitive DER Aggregation for Participation in Wholesale Markets
Source: arXiv:2207.00290 source file (2022-07-01)
Supplement: Supplementary file 2 [file appendix_v0.tex]

\subsection{Property of SFE with capacity limits}

 \begin{lemma} \label{lemma:Range of w}
For every SFE, the price and quantity exists $w$, s.t. the supply function satisfies.   
 \end{lemma}
proof: if reach capacity limits, we can always find one $w$

if not reach capacity limits works

\textcolor{red}{comment $wbf$ in this region can give all SFE}.

\subsection{Proof of Lemma \ref {lemma:SFE_C2} }

 Proof: $\sum_m P_m={\cal D} \Rightarrow \sum_m (R_m- \frac{w_m}{B(\pi)})={\cal D} \Rightarrow \pi=B^{-1}(\frac{\sum_m w_m}{\sum_m R_m-{\cal D}})$.  
Define $F(\mathbf{1}^\intercal \wbf):=B^{-1}(\frac{\sum_m w_m}{\sum_m R_m-{\cal D}})$. So the market clearing price $\pi$ is a function of the sum of the bid-in parameter, i.e. $\pi(\wbf)=F(\mathbf{1}^\intercal \wbf)$.

The wholesale market allocation with $\omega_m$ at SFE has 

$P_m=S_m(\pi(\wbf),w_m)=R_m-\frac{w_m}{B(\pi(\wbf))}\Rightarrow$ $S_m(\pi(\wbf),w_m):= R_m- \frac{(\sum_{j=1}^M R_j - {\cal D})w_m }{\sum_{j=1}^M w_j},$
which is independent of $B(\cdot)$.
 
%  $u_m(\pi)=\frac{\partial S_m(\pi,w_m)}{\partial w_m}=\frac{-1}{B(\pi)}$
 
%  and
 
%  $u_m(\pi(\wbf))=\frac{-1}{B(\pi(\wbf))}=\frac{{\cal D}-\sum_m R_m}{\sum_m w_m}$.

From the capacity limit we have $\underline{P}_m \le P_m\le \bar{P}_m \Rightarrow 
\underline{P}_m \le R_m- \frac{(\sum_{j=1}^M R_j - {\cal D})w_m }{\sum_{j=1}^M w_j}\le \bar{P}_m$. Because $w_m\geq 0, \sum_{j=1}^M w_j\neq 0 \Rightarrow \sum_{j=1}^M w_j> 0$. We have
\[
\underline{w}_m \le w_m\le \bar{w}_m
\]
where $R_{-m}:=\sum_{j\neq m} R_j$.

1. When $B(\cdot)$ is unbounded above, we assume $R_{-m}\geq {\cal D}$, and we have
$ \bar{w}_m=\left\{\begin{matrix}
+\infty,&if~R_{-m}-{\cal D}+\underline{P}_m \le0\\ 
\frac{(R_m-\underline{P}_m)W_{-m}}{R_{-m}-{\cal D}+\underline{P}_m},&if~R_{-m}-{\cal D}+\underline{P}_m>0
\end{matrix}\right., \forall m$ and $\underline{w}_m=\frac{(R_m-\bar{P}_m)W_{-m}}{R_{-m}-{\cal D}+\bar{P}_m}$.

2. $\underline{P}_m \le s_m(\pi(\wbf),w_m)\le \bar{P}_m$.

 Note that to bound the integration in the formulation of $\hat{C}_m(P_m)$, we assume $|P_m| \le |\frac{{\cal D} -\sum_{j=1}^M R_j}{M-1}|, \forall m$ when ${\cal M}< 1$. Meanwhile, $|s_m(\pi(\wbf),w_m)|\le |\frac{{\cal D} -\sum_{j=1}^M R_j}{M-1}|, \forall m$ bounds $\wbf$.

\subsection{Proof of Theorem \ref{thm:SFE_C1} }

At supply function equilibrium, we have 
\begin{equation}
\label{eq:Qprofit}
\begin{array}{lcl}
Q_m(w_m;\wbf_{-m})&=&\pi(\wbf) P_n(\wbf)-C_n(P_n(\wbf))\\
&=&B^{-1}(\frac{\sum_m w_m}{\sum_m R_m-{\cal D}})(R_m- \frac{(\sum_{j=1}^M R_j- {\cal D})w_m }{\sum_{j=1}^M w_j})\\
&&-C_n(R_m- \frac{(\sum_{j=1}^M R_j- {\cal D})w_m }{\sum_{j=1}^M w_j}).
% \left\{\begin{matrix}
%   d^-,& if~  g\geq d^-\\ 
%   d^+,& if~  g\le d^+  
% \end{matrix}\right.,
\end{array}
\end{equation}

\begin{lemma} \label{lemma:SFE_w2}
If $\wbf$ is a supply function equilibrium (Nash equilibrium), then at least two coordinates of $\wbf$ are positive.  
 \end{lemma}
 {\em Proof:} Fix a wholesale market participant $m$, and suppose $\wbf_{-m} = \mathbf{0}$. From (\ref{eq:Qprofit}), the payoff to  $m$ is then:
\beq
\begin{array}{lcl}
 Q_m(w_m;\mathbf{0})&=&B^{-1}(\frac{ w_m}{\sum_m R_m-{\cal D}})( {\cal D}-R_{-m})\\
 &&-C_n( {\cal D}-R_{-m}).
\end{array}
\eeq
According to Assumption \ref{assump:SFE_C2}, we have $R_{-m}\geq {\cal D} $.  Besides, $B(\cdot)$ is strictly increasing. So, participant $m$   would like to submit an arbitrarily low (but positive) bid $w_m$ to minimize the market clearing price. Since this holds for every participant, we conclude that at least two coordinates of $\wbf$ must be positive.

 \begin{lemma} \label{lemma:SFE_M3}
If $M =2$, then no supply function equilibrium (Nash equilibrium) exists. 
 \end{lemma}
  {\em Proof:} Suppose that $(w_1,w_2)$ is a Nash equilibrium. Then by Lemma \ref{lemma:SFE_w2}, $w_1 > 0$ and $w_2 > 0$; and in this case the payoff to  participant $m$ as a function of $w_1 \geq 0$ is:
  \begin{equation}
\begin{array}{lcl}
Q_1(w_1;w_2)&=&B^{-1}(\frac{w_1+w_2}{R_1+R_2-{\cal D}})({\cal D}-R_2- \frac{(R_1+R_2- {\cal D})w_2 }{ w_1+w_2})\\
&&-C_n({\cal D}-R_2- \frac{(R_1+R_2- {\cal D})w_2 }{ w_1+w_2}).
% \left\{\begin{matrix}
%   d^-,& if~  g\geq d^-\\ 
%   d^+,& if~  g\le d^+  
% \end{matrix}\right.,
\end{array}
\end{equation}
We have $R_m\geq {\cal D} ,\forall m=1,2$ and $B(\cdot)$ is strictly increasing. So, the preceding expression is strictly increasing in $w_1$, and $(w_1,w_2)$ could not have been a Nash equilibrium. Thus no Nash equilibrium exists if $N = 2$.

{\em Step 1: Necessary and Sufficient Nash Equilibrium Condition:} We argue in this step that the vector $\wbf$ is a Nash equilibrium if and only if at least two components of $\wbf$ are positive, $\underline{w}_m \le w_m\le \bar{w}_m,\forall m$, and the following conditions hold:

Thus we must maximize $Q_m(w_m;\wbf_{-m})$ in (\ref{eq:Qprofit}) over $\underline{w}_m \le w_m\le \bar{w}_m$, and satisfy the following first order optimality conditions when ${\cal M}>0$:
\beq
\begin{array}{lcl}\label{deriativeQfinal1}
\frac{\partial^- C_m(S_m(\pi(\wbf),w_m))}{\partial P_m}(1+\frac{S_m(\pi(\wbf),w_m)}{-D+R_{-m}})\le {\cal M} \pi(\wbf),&\\
if~ \underline{w}_m \le w_m< \bar{w}_m &\\
\frac{\partial^+ C_m(S_m(\pi(\wbf),w_m))}{\partial P_m}(1+\frac{P_m(\pi(\wbf),w_m)}{-D+R_{-m}})\ge {\cal M} \pi(\wbf),&\\
if~ \underline{w}_m < w_m\le \bar{w}_m &
\end{array}
\eeq

the following first order optimality conditions when ${\cal M}<0$:
\beq
\begin{array}{lcl}\label{deriativeQfinal2}
\frac{\partial^- C_m(S_m(\pi(\wbf),w_m))}{\partial P_m}(1+\frac{S_m(\pi(\wbf),w_m)}{-D+R_{-m}})\le {\cal M} \pi(\wbf),&\\
if~ \underline{w}_m < w_m\le \bar{w}_m &\\
\frac{\partial^+ C_m(S_m(\pi(\wbf),w_m))}{\partial P_m}(1+\frac{P_m(\pi(\wbf),w_m)}{-D+R_{-m}})\ge {\cal M} \pi(\wbf),&\\
if~ \underline{w}_m \le w_m < \bar{w}_m &
\end{array}
\eeq
Detailed derivation is shown below:
$w_m$ maximize $Q_m(w_m;\wbf_{−m})$ in (\ref{eq:Qprofit}) and satisfy F.O.C.:
\beq
\begin{array}{lcl}\label{deriativeQ1}
\frac{\partial^+ Q_m(w_m;\wbf_{-m})}{\partial w_m}\le 0, if~ \underline{w}_m \le w_m< \bar{w}_m\\
\frac{\partial^- Q_m(w_m;\wbf_{-m})}{\partial w_m}\ge 0, if~ \underline{w}_m < w_m\le \bar{w}_m
\end{array}
\eeq

Recalling the expression for $\pi(\wbf)=F(\mathbf{1}^\intercal \wbf)=B^{-1}(\frac{\sum_m w_m}{\sum_m R_m-{\cal D}})$ in Lemma \ref {lemma:SFE_C2} and Lemma \ref {lemma:SFE_C1}, with assumption  $B(\pi)B^{-1'}(B(\pi))={\cal M}\pi$, after multiplying through by $\pi(\wbf)$ the preceding

Define $v_m:=\frac{\partial F(\cdot)}{\partial w_m}=\frac{B^{-1'}(\frac{\sum_m w_m}{\sum_m R_m-{\cal D}})}{\sum_m R_m-{\cal D}}$.

Define
 $h_m(w_m):=\frac{d S_m(\cdot)}{d w_m}=\frac{({\cal D}-\sum_{j=1}^M R_j)W_{-m}}{(\sum_{j=1}^M w_j)^2}$.  According to Assumption \ref{assump:SFE_C2}, we have $R_{-m}\geq {\cal D} $. So $h_m < 0, \forall m$ 
 
 $W_{-m}:=\sum_{j\neq m} w_j, R_{-m}:=\sum_{j\neq m} R_j$
 
\textcolor{red}{show computation procedure with the above defined function.}

\beq
\begin{array}{lcl}\label{deriativeQ}
\frac{\partial^- C_m(S_m(\pi(\wbf),w_m))}{\partial P_m}\frac{W_{-m}}{\sum_{j=1}^{M} w_j}\le \frac{{\cal M}(R_{-m}-{\cal D})}{\sum_{j=1}^{M} R_j-{\cal D}}\pi(\wbf),&\\
if~ \underline{w}_m \le w_m< \bar{w}_m &\\
\frac{\partial^+ C_m(S_m(\pi(\wbf),w_m))}{\partial P_m}\frac{W_{-m}}{\sum_{j=1}^{M} w_j}\ge \frac{{\cal M}(R_{-m}-{\cal D})}{\sum_{j=1}^{M} R_j-{\cal D}} \pi(\wbf),&\\
if~ \underline{w}_m < w_m\le \bar{w}_m &
\end{array}
\eeq
 
 We now note that by definition, we have:
\beq
\begin{array}{lcl}
\frac{W_{-m}}{\sum_{j=1}^M w_j}&=&1-\frac{w_{m}}{\sum_{j=1}^M w_j}\\
&&=1-\frac{(R_m-S_m(\pi(\wbf),w_m))B(\pi)}{B(\pi)\sum_m((R_m-S_m(\pi(\wbf),w_m)))}\\
&&=\frac{(R_{-m}-{\cal D}+S_m(\pi(\wbf),w_m))}{\sum_{j=1}^MR_j-{\cal D}}
\end{array}
\eeq
 
Substituting into (\ref{deriativeQ}) and simplifying yields (\ref{deriativeQfinal1}) and (\ref{deriativeQfinal2}).

 {\em Step 2: Existence and Uniqueness of an Optimal Solution to (\ref{eq:SFE_thmC}):}
  We first argue that $\hat{C}_m(P_m)$ is continuous, strictly convex and strictly increasing over $\underline{P}_m \le P_m\le \bar{P}_m$. From the definition of $\hat{C}_m(P_m)$ we have
\beq
\begin{array}{lcl}\label{CEquivelentderiative}
\frac{\partial^- \hat{C}_m(P_m)}{\partial P_m}=\frac{\partial^- C_m(P_m)}{\partial P_m}(1+\frac{P_m}{-D+R_{-m}})\le {\cal M}\pi(\wbf),&\\
if~\underline{P}_m < P_m\le \bar{P}_m &\\
\frac{\partial^+ \hat{C}_m(P_m)}{\partial P_m}=\frac{\partial^+ C_m(P_m)}{\partial P_m}(1+\frac{P_m}{-D+R_{-m}})\ge {\cal M}\pi(\wbf),&\\
if~ \underline{P}_m \le P_m< \bar{P}_m &
\end{array}
\eeq

Since $C_m$ is strictly increasing and convex, for any $\underline{P}_m \le P_m\le \bar{P}_m$, we have
\beq
\begin{array}{lcl}
0\le \frac{\partial^+ \hat{C}_m(P_m)}{\partial P_m}<\frac{\partial^- \hat{C}_m(\bar{P}_m)}{\partial P_m}<\frac{\partial^+ \hat{C}_m(\bar{P}_m)}{\partial P_m}
\end{array}
\eeq
This guarantees that $\hat{C}_m(P_m)$  is strictly increasing and strictly convex over $\underline{P}_m \le P_m\le \bar{P}_m$,.

 {\em Step 3: Necessary and Sufficient Optimality Condition for the Problem in (7):}
( \ref{CEquivelentderiative}) coincides with (\ref{deriativeQfinal1}) and (\ref{deriativeQfinal2}).
 
%  {\em Step 4: Uniqueness of Nash Equilibrium Under an Addi- tional Assumption: W}
