# Supplementary material for: Competitive DER Aggregation for Participation in Wholesale Markets
Source: arXiv:2207.00290 source file (2022-07-01)
Supplement: Supplementary file 3 [file appendixProofTHM1_v0.tex]

KKT conditions of (\ref{eq:DERAsurplus_LnGP}) are
\bea\label{eq:DERA_KKT}
\begin{array}{lrl}
1-\lambda^*_n=0, \forall n,\\
V'_{kn}(d^*_{kn})-\pi_{\mbox{\tiny LMP}}-\underline{\mu}^*_{kn}+\bar{\mu}^*_{kn} =0,\forall n, k,\\
\lambda^*_n({\cal K}_n(g_n)- U_n(\dbf^*_n)+\omega^*_n)=0,\forall n,\\
\underline{\mu}^*_{kn}(\underline{d}_{kn}- d_{kn} )=0,\forall n, k,\\
\bar{\mu}^*_{kn}(d_{kn} -\bar{d}_{kn})=0,\forall n, k,\\
{\cal K}_n(g_n)\le U_n(\dbf^*_n)-\omega^*_n,\forall n\\
\underline{\dbf_n} \preceq  \dbf_n \preceq  \bar{\dbf_n},\forall n.
\end{array}
\eea

So the ${\cal K}$-competitive constraint is always binding, and the optimal scheduling and payment of (\ref{eq:DERAsurplus_LnGP}) is  
\begin{align}
% d^*_{kn}&= \max \{\underline{d}_k,\min \{V_{kn}^{-1}(\pi_{\mbox{\tiny LMP}} ),\bar{d}_k\}\}\nn\\
d^*_{kn}&= \begin{cases}
\bar{d}_{kn}&if~V_{kn}^{-1}(\pi_{\mbox{\tiny LMP}})\geq \bar{d}_{kn} \\ 
V_{kn}^{-1}(\pi_{\mbox{\tiny LMP}}),&if~\underline{d}_{kn} \le V_{kn}^{-1}(\pi_{\mbox{\tiny LMP}}) \le \bar{d}_{kn}\\
\underline{d}_{kn},&if~ V_{kn}^{-1}(\pi_{\mbox{\tiny LMP}}) \le \underline{d}_{kn}
\end{cases},\nn\\
\omega^{*}_n&(\dbf_n^*,g_n)= U_n(\dbf_n^*)-{\cal K}_n(g_n).\nn 
\end{align}
