# Supplementary material for: Competitive DER Aggregation for Participation in Wholesale Markets
Source: arXiv:2207.00290 source file (2022-07-01)
Supplement: Supplementary file 5 [file appendixProofTHM2_v0.tex]

% (\ref{eq:ProfitMaxDirect}) is the profit maximization of the individual prosumer when it directly participate in the wholesale market.

Solving (\ref{eq:wholesaleDiret}) we have $\dbf^{\mbox{\tiny Direct}}_n, p^{\mbox{\tiny Direct}}_r$ and we know that $\pi_{\mbox{\tiny LMP}}=\lambda^*$. By KKT conditions of  (\ref{eq:wholesaleDiret}), we know 
$$d^{\mbox{\tiny Direct}}_{kn}=\max \{\underline{d}_k,\min \{V_{kn}^{-1}(\pi_{\mbox{\tiny LMP}} ),\bar{d}_k\}\}=d^*_{kn}, \forall k, n,$$
where in $d^*_{kn}$ is computed with (\ref{eq:DERAFixRateGP}). So $\dbf^{*}_n$ is the same as the optimal consumption of the prosumer $n$ when it directly participates in the wholesale market with individual profit maximization (\ref{eq:ProfitMaxDirect}) and market clearing problem  (\ref{eq:wholesaleDiret}).

To satisfy the power balance constraints with social welfare maximization, we have  $p^{\mbox{\tiny Direct}}_l=p^*_l, \forall l$. So 
\beq
\begin{array}{lcl}
S_{{\cal W}}&:=&\sum_nU_n(\dbf^{\mbox{\tiny Direct}}_n)-\sum_lC_l(p^{\mbox{\tiny Direct}}_l)\\
&=&\sum_nU_n(\dbf^*_n)-\sum_lC_l(p^*_l)\\
&=& S_{\tiny {\cal W}\mbox{-DERA}}.
\end{array}
\eeq

follows directly the KKT conditions of (\ref{eq:wholesaleDiret}) and (\ref{eq:ProfitMaxDirect}), from which we have, $\hat{\dbf}_n$, the optimal consumption of the prosumer $n$ the same as $\dbf^{*}_n$  in (\ref{eq:DERAFixRateGP}). Therefore, when prosumers directly participate in the wholesale market, both the optimal wholesale market dispatch and the optimal social welfare are the same as those when prosumers indirectly participate in the wholesale electricity market through a DERA.
